# Supplementary material for: ConceptBed: Evaluating Concept Learning Abilities of Text-to-Image Diffusion Models
Source: arXiv:2306.04695 source file (2024-02-22)
Supplement: Supplementary file 1 [file accecibility.tex]

\begin{table*}[h]
    \centering    
    \begin{tabular}{l l}
        \textbf{Name} & \textbf{Link} \\
        \midrule
        Project Page: & \href{https://conceptbed.github.io}{https://conceptbed.github.io} \\
        Code: & \href{https://github.com/ConceptBed/evaluations}{https://github.com/ConceptBed/evaluations} \\
        Data: & \href{https://conceptbed.github.io/data.html}{https://conceptbed.github.io/data.html} \\
        Results Explorer: & \href{https://conceptbed.github.io/explorer.html}{https://conceptbed.github.io/explorer.html} \\
        \bottomrule
    \end{tabular}%
\end{table*}
